# Supplementary material for: Apparatus for Optical-Atomic System Integration & Calibration: 1 atm to 1$\times$10$^{-11}$ Torr in 24h
Source: arXiv:2407.13129 source file (2024-07-18)
Supplement: Supplementary file 1 [file supplemental.tex]

\begin{appendix}

\section{\label{app:firstsection}section title here}
\vspace{-4pt}

\end{appendix}
